# Supplementary material for: Communication-Efficient Distributed Learning with Local Immediate Error Compensation
Source: arXiv:2402.11857 source file (2024-02-19)
Supplement: Supplementary file 1 [file appendix.tex]

\section{Proofs of Theoretical Results}
Now we begin the proof. Define the virtual sequence $\{\hat{x}_t\}$ as follows:
\begin{equation}
    \hat{x}_{t+1} = \hat{x}_t- \frac{1}{N} \sum_{i=1}^N \eta \nabla f_i(x_t^i, \xi_t^i). \nonumber
\end{equation}
Then we have that
\begin{lemma}\label{lemma6}
For $\{\hat{x}_t\}$ and $\{\Bar{x}_t\}$ in Algorithm~\ref{LIEC}
\begin{equation}
    \Bar{x}_t-\hat{x}_t = \eta e_t.
\end{equation}
\end{lemma}

\begin{proof}
According to the update rule, we can obtain that
\begin{eqnarray}
\Bar{x}_t-\hat{x}_t &=& \bigg(x_0-\sum_{\tau=0}^{t-1} \frac{1}{N} \sum_{i=1}^N \eta (p_\tau-p_\tau^i+\nabla f_i(x_\tau^i, \xi_\tau^i))\bigg)-\bigg(x_0-\sum_{\tau=0}^{t-1}\frac{1}{N} \sum_{i=1}^N \eta \nabla f_i(x_\tau^i, \xi_\tau^i)\bigg) \nonumber \\
&&= \frac{1}{N} \sum_{\tau=0}^{t-1} \sum_{i=1}^N \eta (p_\tau^i-p_\tau) \nonumber \\
&&= \frac{1}{N} \sum_{\tau=0}^{t-1} \sum_{i=1}^N \eta (v_\tau-e_\tau+e_{\tau+1}-v_\tau) \nonumber \\
&&= \eta e_t \nonumber
\end{eqnarray}
\end{proof}

\textbf{Proof of Lemma~\ref{lemma1}}
\begin{proof}
When $(t+1) \% \lfloor \frac{1}{\delta} \rfloor=0$, we have $\|e_t\|=0$. We focus on the iterations where $(t+1) \% \lfloor \frac{1}{\delta} \rfloor\neq0$.
\begin{eqnarray}\label{lemma1_1}
\mathbb{E}\|e_t\|^2 &=& \mathbb{E}\|v_{t-1}-\mathcal{C}_\delta(v_{t-1})\|^2 \nonumber \\
&\leq& (1-\delta) \mathbb{E}\|v_{t-1}\|^2 \nonumber \\
\end{eqnarray}
where the first inequality comes from Definition 1. Further, by the Young's Inequality, we have
\begin{eqnarray}\label{lemma1_2}
\mathbb{E}\|e_t\|^2 &\leq& (1-\delta)(1+\beta) \mathbb{E}\|e_{t-1}\|^2 + (1-\delta)(1+1/\beta) \mathbb{E}\|\frac{1}{N} \sum_{i=1}^N p_{t-1}^i\|^2 \nonumber \\
&\leq& (1-\delta)(1+\beta) \mathbb{E}\|e_{t-1}\|^2 + \frac{(1-\delta)(1+1/\beta)}{N} \sum_{i=1}^N \mathbb{E}\|\mathcal{C}_\delta (\nabla f_i(x_{t-1}^i,\xi_{t-1}^i))\|^2 \nonumber \\
&\leq& (1-\delta)(1+\beta) \mathbb{E}\|e_{t-1}\|^2 +\frac{(1-\delta)(1+1/\beta)}{N} \sum_{i=1}^N \mathbb{E}\|\mathcal{C}_\delta (\nabla f_i(x_{t-1}^i,\xi_{t-1}^i)\nonumber \\
&&-\nabla f_i(x_{t-1}^i,\xi_{t-1}^i)+\nabla f_i(x_{t-1}^i,\xi_{t-1}^i))\|^2 \nonumber \\
&\leq& (1-\delta)(1+\beta) \mathbb{E}\|e_{t-1}\|^2 + \frac{2(1-\delta)(2-\delta)(1+1/\beta)}{N} \sum_{i=1}^N \mathbb{E}\|\nabla f_i(x_{t-1}^i,\xi_{t-1}^i)\|^2 \nonumber \\
&\leq& (1-\delta)(1+\beta) \mathbb{E}\|e_{t-1}\|^2 + 2(1-\delta)(2-\delta)(1+1/\beta) M^2 \nonumber \\
&\leq& \frac{2(1-\delta)(2-\delta)(1+1/\beta) M^2}{1-(1-\delta)(1+\beta)} \nonumber \\
&\leq& \frac{8(1-\delta)(2-\delta)M^2}{\delta^2}.
\end{eqnarray}
The second inequality comes from the Cauchy's Inequality. The fifth inequality follows from Assumption~\ref{assu3}. The last inequality holds by setting $\beta = \frac{\delta}{2(1-\delta)}$.
\end{proof}

\textbf{Proof of Lemma~\ref{lemma2}}
\begin{proof}
We define $t'<t$ as the largest iteration index that is a multiple of $\lfloor \frac{1}{\delta} \rfloor$. According to the update rule, we have that
\begin{eqnarray}
\Bar{x}_t-x_t^i &=& \Bar{x}_{t'} - \eta \frac{1}{N}\sum_{j=1}^N \sum_{\tau=t'}^{t-1} (p_\tau-p_\tau^j+\nabla f_i(x_\tau^j,\xi_\tau^j))-(x_{t'}^i-\eta \sum_{\tau=t'}^{t-1}(p_\tau-p_\tau^i+\nabla f_i(x_\tau^i,\xi_\tau^i))) \nonumber \\
&=& \eta \sum_{\tau=t'}^{t-1}(\nabla f_i(x_\tau^i,\xi_\tau^i)-\mathcal{C}_\delta(\nabla f_i(x_\tau^i,\xi_\tau^i))-(\frac{1}{N}\sum_{j=1}^N \nabla f_i(x_\tau^j,\xi_\tau^j)-\mathcal{C}_\delta(\nabla f_i(x_\tau^j,\xi_\tau^j)))). \nonumber
\end{eqnarray}
So we have that
\begin{eqnarray}\label{lemma2_1}
&&\sum_{i=1}^N \mathbb{E}\|\Bar{x}_t-x_t^i\|^2 \nonumber \\
&=& \eta^2  \sum_{i=1}^N \mathbb{E}\|\sum_{\tau=t'}^{t-1}\nabla f_i(x_\tau^i,\xi_\tau^i)-\mathcal{C}_\delta(\nabla f_i(x_\tau^i,\xi_\tau^i))-(\frac{1}{N}\sum_{j=1}^N \nabla f_i(x_\tau^j,\xi_\tau^j)-\mathcal{C}_\delta(\nabla f_i(x_\tau^j,\xi_\tau^j)))\|^2 \nonumber \\
&=& \eta^2 \bigg(\sum_{i=1}^N \mathbb{E}\|\sum_{\tau=t'}^{t-1}\nabla f_i(x_\tau^i,\xi_\tau^i)-\mathcal{C}_\delta(\nabla f_i(x_\tau^i,\xi_\tau^i))\|^2 \nonumber \\
&&-\frac{1}{N}\mathbb{E}\|\sum_{\tau=t'}^{t-1} \sum_{j=1}^N \nabla f_i(x_\tau^j,\xi_\tau^j)-\mathcal{C}_\delta(\nabla f_i(x_\tau^j,\xi_\tau^j))\|^2\bigg) \nonumber \\
&\leq& \eta^2 \sum_{i=1}^N \mathbb{E}\|\sum_{\tau=t'}^{t-1}\nabla f_i(x_\tau^i,\xi_\tau^i)-\mathcal{C}_\delta(\nabla f_i(x_\tau^i,\xi_\tau^i))\|^2 \nonumber \\
&\leq& \eta^2 (t-t')\sum_{i=1}^N \sum_{\tau=t'}^{t-1} \mathbb{E}\|\nabla f_i(x_\tau^i,\xi_\tau^i)-\mathcal{C}_\delta(\nabla f_i(x_\tau^i,\xi_\tau^i))\|^2
\end{eqnarray}
where the last inequality comes from the Cauchy's Inequality. Then according to Definition 1, we have
\begin{eqnarray}\label{lemma2_2}
\sum_{i=1}^N \mathbb{E}\|\Bar{x}_t-x_t^i\|^2 &\leq& (1-\delta)\eta^2 (t-t')\sum_{i=1}^N \sum_{\tau=t'}^{t-1} \mathbb{E}\|\nabla f_i(x_\tau^i,\xi_\tau^i)\|^2 \nonumber \\
&\leq& (1-\delta)\eta^2 (t-t')^2 N M^2 \nonumber \\
&\leq& \frac{1-\delta}{\delta^2}\eta^2 N M^2
\end{eqnarray}
where the second inequality follows from Assumption~\ref{assu3}. The last inequality holds because $t-t' \leq \lfloor \frac{1}{\delta} \rfloor \leq \frac{1}{\delta}$. 
\end{proof}

\textbf{Proof of Lemma~\ref{lemma3}}
\begin{proof}
\begin{eqnarray}\label{lemma7_1}
&&\mathbb{E}\|\frac{1}{N} \sum_{i=1}^N \nabla f_i(x_t^i, \xi_t^i)\|^2 \nonumber \\
&=& \mathbb{E}\|\frac{1}{N} \sum_{i=1}^N \nabla f_i(x_t^i, \xi_t^i)-\nabla f_i(x_t^i)+\nabla f_i(x_t^i)-\nabla f_i(\Bar{x}_t)+\nabla f_i(\Bar{x}_t)\|^2 \nonumber \\
&=& \mathbb{E}\|\frac{1}{N} \sum_{i=1}^N \nabla f_i(x_t^i, \xi_t^i)-\nabla f_i(x_t^i)\|^2+\mathbb{E}\|\frac{1}{N} \sum_{i=1}^N\nabla f_i(x_t^i)-\nabla f_i(\Bar{x}_t)+\nabla f_i(\Bar{x}_t)\|^2 \nonumber \\
&=& \frac{1}{N^2} \sum_{i=1}^N \mathbb{E}\|\nabla f_i(x_t^i, \xi_t^i)-\nabla f_i(x_t^i)\|^2+\mathbb{E}\|\frac{1}{N} \sum_{i=1}^N\nabla f_i(x_t^i)-\nabla f_i(\Bar{x}_t)+\nabla f_i(\Bar{x}_t)\|^2, \nonumber \\
\end{eqnarray}
where the second and third equality hold because ${\xi_t^{i}}'s$ are independent and $\mathbb{E}[\nabla f_i(x_t^i, \xi_t^i)]=\nabla f_i(x_t^i)$. Further, we have

\begin{eqnarray}
&&\mathbb{E}\|\frac{1}{N} \sum_{i=1}^N \nabla f_i(x_t^i, \xi_t^i)\|^2 \nonumber \\
&\leq& \frac{\sigma^2}{N} + 2\mathbb{E}\|\frac{1}{N} \sum_{i=1}^N\nabla f_i(x_t^i)-\nabla f_i(\Bar{x}_t)\|^2+2\mathbb{E}\|\nabla f(\Bar{x}_t)\|^2 \nonumber \\
&\leq& \frac{\sigma^2}{N} + \frac{2L^2}{N}\sum_{i=1}^N\mathbb{E}\|x_t^i-\Bar{x}_t\|^2+2\mathbb{E}\|\nabla f(\Bar{x}_t)\|^2.
\end{eqnarray}
The first inequality comes from Assumption~\ref{assu2} and the fact that $\|a+b\|^2 \leq 2\|a\|^2+2\|b\|^2$. The last inequality follows from the Cauchy's Inequality and Assumption~\ref{assu1}. %Substituting Lemma~\ref{lemma7} into (\ref{lemma8_1}) yields the result.
\end{proof}

\textbf{Proof of Theorem~\ref{theo_1}}
\begin{proof}
According to the $L$-smoothness of $f(x)$, we have that
\begin{eqnarray}\label{theo1_1}
\mathbb{E} [f(\Hat{x}_{t+1})] &\leq& \mathbb{E} [f(\Hat{x}_t)]+\mathbb{E} \langle \nabla f(\Hat{x}_t), \Hat{x}_{t+1}-\Hat{x}_t \rangle + \frac{L}{2}\mathbb{E} \|\Hat{x}_{t+1}-\Hat{x}_t\|^2 \nonumber \\
&=& \mathbb{E} [f(\Hat{x}_t)]-\eta \mathbb{E} \langle \nabla f(\Hat{x}_t), \frac{1}{N} \sum_{i=1}^{N} \nabla f_i(x_t^i,\xi_t^i) \rangle + \frac{\eta^2 L}{2}\mathbb{E} \|\frac{1}{N} \sum_{i=1}^{N} \nabla f_i(x_t^i,\xi_t^i)\|^2 \nonumber \\
&=& \mathbb{E} [f(\Hat{x}_t)]-\eta \mathbb{E} \langle \nabla f(\Hat{x}_t), \frac{1}{N} \sum_{i=1}^{N} \nabla f_i(x_t^i) \rangle + \frac{\eta^2 L}{2}\mathbb{E} \|\frac{1}{N} \sum_{i=1}^{N} \nabla f_i(x_t^i,\xi_t^i)\|^2.
\end{eqnarray}
Note that
\begin{eqnarray}
    &&\langle \nabla f(\Hat{x}_t), \frac{1}{N} \sum_{i=1}^{N} \nabla f_i(x_t^i) \rangle \nonumber \\
    &=& \langle \nabla f(\Hat{x}_t), \frac{1}{N} \sum_{i=1}^{N} \nabla f_i(\Bar{x}_t) \rangle - \langle \nabla f(\Hat{x}_t),\frac{1}{N} \sum_{i=1}^{N} \nabla f_i(\Bar{x}_t)- \nabla f_i(x_t^i) \rangle \nonumber \\
    &=& \langle \nabla f(\Hat{x}_t), \nabla f(\Bar{x}_t) \rangle - \langle \nabla f(\Hat{x}_t),\frac{1}{N} \sum_{i=1}^{N} \nabla f_i(\Bar{x}_t)- \nabla f_i(x_t^i) \rangle. \nonumber
\end{eqnarray}
So we have that
\begin{eqnarray}
\mathbb{E} [f(\Hat{x}_{t+1})] &\leq& \mathbb{E} [f(\Hat{x}_t)]-\eta \mathbb{E} \langle \nabla f(\Hat{x}_t), \nabla f(\Bar{x}_t) \rangle + \eta \mathbb{E} \langle \nabla f(\Hat{x}_t),\frac{1}{N} \sum_{i=1}^{N} \nabla f_i(\Bar{x}_t)- \nabla f_i(x_t^i) \rangle\nonumber \\
&&+ \frac{\eta^2 L}{2}\mathbb{E} \|\frac{1}{N} \sum_{i=1}^{N} \nabla f_i(x_t^i,\xi_t^i)\|^2 \nonumber \\
&\leq& \mathbb{E} [f(\Hat{x}_t)]-\frac{\eta}{2} \mathbb{E} (\|\nabla f(\Hat{x}_t)\|^2+\|\nabla f(\Bar{x}_t)\|^2-\|\nabla f(\Hat{x}_t)-\nabla f(\Bar{x}_t)\|^2)\nonumber \\
&&+ \frac{\eta}{2} \mathbb{E} (\|\nabla f(\Hat{x}_t)\|^2+\|\frac{1}{N} \sum_{i=1}^{N} \nabla f_i(\Bar{x}_t)- \nabla f_i(x_t^i)\|^2) + \frac{\eta^2 L}{2}\mathbb{E} \|\frac{1}{N} \sum_{i=1}^{N} \nabla f_i(x_t^i,\xi_t^i)\|^2, \nonumber \\
\end{eqnarray}
where the last inequality comes from the fact that $2\langle a, b \rangle \leq \|a\|^2 + \|b\|^2$. Further, we have
\begin{eqnarray}\label{theo1_2}
\mathbb{E} [f(\Hat{x}_{t+1})] &\leq&  \mathbb{E} [f(\Hat{x}_t)] - \frac{\eta}{2}\mathbb{E} \|\nabla f(\Bar{x}_t)\|^2 + \frac{\eta L^2}{2}\mathbb{E} \|\Hat{x}_t-\Bar{x}_t\|^2  \nonumber \\
&&+ \frac{\eta L^2}{2N}  \sum_{i=1}^N \mathbb{E} \|\Bar{x}_t-x_t^i\|^2 + \frac{\eta^2 L}{2}\mathbb{E} \|\frac{1}{N} \sum_{i=1}^{N} \nabla f_i(x_t^i,\xi_t^i)\|^2 \nonumber \\
&=&  \mathbb{E} [f(\Hat{x}_t)] - \frac{\eta}{2}\mathbb{E} \|\nabla f(\Bar{x}_t)\|^2 + \frac{\eta^3 L^2}{2}\mathbb{E} \|e_t\|^2 + \frac{\eta L^2}{2N}  \sum_{i=1}^N \mathbb{E} \|\Bar{x}_t-x_t^i\|^2 \nonumber \\
&&+ \frac{\eta^2 L}{2}\mathbb{E} \|\frac{1}{N} \sum_{i=1}^{N} \nabla f_i(x_t^i,\xi_t^i)\|^2,
\end{eqnarray}
where the inequality follows from Assumption 1 and the equality comes from Lemma~\ref{lemma6}.
Summing up (\ref{theo1_2}) over $\{0, 1, ..., T-1\}$ and ignoring the $\mathbb{E} \|\nabla f(\Hat{x}_t)\|^2$ term yield that
\begin{eqnarray}\label{theo1_3}
    \frac{\eta}{2}\sum_{t=0}^{T-1}\mathbb{E} \|\nabla f(\Bar{x}_t)\|^2 &\leq& f(x_0)-f(x^*) + \frac{\eta^3 L^2}{2} \sum_{t=0}^{T-1} \mathbb{E} \|e_t\|^2 + \frac{\eta L^2}{2N}  \sum_{t=0}^{T-1}  \sum_{i=1}^N \mathbb{E}\|\Bar{x}_t-x_t^i\|^2 \nonumber \\
    &&+ \frac{\eta^2 L}{2}\sum_{t=0}^{T-1} \mathbb{E} \|\frac{1}{N} \sum_{i=1}^{N} \nabla f_i(x_t^i,\xi_t^i)\|^2.
\end{eqnarray}
Substituting Lemma~\ref{lemma1}-\ref{lemma3} into (\ref{theo1_3}) yields that
\begin{eqnarray}\label{theo1_4}
    \frac{\eta}{2}\sum_{t=0}^{T-1}\mathbb{E} \|\nabla f(\Bar{x}_t)\|^2 &\leq& f(x_0)-f(x^*) + \frac{4(1-\delta)(2-\delta)\eta^3 L^2 T M^2}{\delta^2} + \frac{(1-\delta)\eta^3 L^2 T M^2}{2\delta^2} \nonumber \\
    &&+ \frac{\eta^2 L}{2}(\frac{T \sigma^2}{N}+\frac{2(1-\delta)\eta^2 L^2 T M^2}{\delta^2}+2\sum_{t=0}^{T-1} \mathbb{E}\|\nabla f(\Bar{x}_t)\|^2) \nonumber \\
    &=& f(x_0)-f(x^*) + \frac{(17+2\eta L)(1-\delta)\eta^3 L^2 T M^2}{2\delta^2} +\frac{\eta^2 L T \sigma^2}{2N} \nonumber \\
    &&+\eta^2 L \sum_{t=0}^{T-1} \mathbb{E}\|\nabla f(\Bar{x}_t)\|^2\nonumber.
\end{eqnarray}
Further we can obtain that
\begin{equation}\label{theo1_5}
    (\frac{\eta}{2}-\eta^2 L)\sum_{t=0}^{T-1}\mathbb{E} \|\nabla f(\Bar{x}_t)\|^2 \leq f(x_0)-f(x^*) + \frac{(17+2\eta L)(1-\delta)\eta^3 L^2 T M^2}{2\delta^2} +\frac{\eta^2 L T \sigma^2}{2N}.
\end{equation}
Dividing by $\frac{\eta T}{2}$ on both sides of (\ref{theo1_5}) and combined with $\eta L < \frac{1}{2}$ yield that
\begin{equation}
    \frac{1-2\eta L}{T}\sum_{t=0}^{T-1}\mathbb{E} \|\nabla f(\Bar{x}_t)\|^2 \leq \frac{2(f(x_0)-f(x^*))}{\eta T} + \frac{18(1-\delta)\eta^2 L^2 M^2}{\delta^2} +\frac{\eta L \sigma^2}{N}.
\end{equation}
\end{proof}

\textbf{Proof of Corollary~\ref{coro_1}}
\begin{proof}
Consider that we set
\begin{equation}
    \eta = \frac{1}{\sqrt{\frac{T}{N}}+4L+\frac{(1-\delta)^{1/2} T^{1/3}}{\delta^{2/3}}},
\end{equation}
then for the second term on the right side of Theorem~\ref{theo_1}, we have
\begin{equation}
    \frac{18(1-\delta)\eta^2 L^2 M^2}{\delta^2} \leq \frac{18(1-\delta)L^2 M^2}{\delta^2}\frac{1}{(\frac{(1-\delta)^{1/2} T^{1/3}}{\delta^{2/3}})^2} = O\bigg(\frac{1}{\delta^{2/3} T^{2/3}}\bigg). \nonumber
\end{equation}
For the third term, we have
\begin{equation}
    \frac{\eta L \sigma^2}{N} \leq \frac{L \sigma^2}{N\sqrt{\frac{T}{N}}} = O\bigg(\frac{1}{\sqrt{NT}}\bigg).
\end{equation}
Finally, for the first term, we have
\begin{equation}
    \frac{2(f(x_0)-f(x^*))}{\eta T} = \frac{2(f(x_0)-f(x^*))(\sqrt{\frac{T}{N}}+4L+\frac{(1-\delta)^{1/2} T^{1/3}}{\delta^{2/3}})}{T} = O\bigg(\frac{1}{\sqrt{NT}}+\frac{1}{T}+\frac{1}{\delta^{2/3} T^{2/3}}\bigg). \nonumber
\end{equation}
Thus we complete the proof.
\end{proof}

\textbf{Proof of Lemma~\ref{lemma4}}
\begin{proof}
Similar to the proof of Lemma~\ref{lemma1}, we have that
\begin{eqnarray}\label{lemma4_1}
\mathbb{E}\|e_t\|^2 &=& \mathbb{E}\|v_{t-1}-\mathcal{C}_\delta(v_{t-1})\|^2 \nonumber \\
&\leq& (1-\delta) \mathbb{E}\|v_{t-1}\|^2 \nonumber \\
&\leq& (1-\delta)(1+\beta) \mathbb{E}\|e_{t-1}\|^2 + (1-\delta)(1+1/\beta) \mathbb{E}\|\frac{1}{N} \sum_{i=1}^N p_{t-1}^i\|^2 \nonumber \\
&=& (1-\delta)(1+\beta) \mathbb{E}\|e_{t-1}\|^2 + \frac{(1-\delta)(1+1/\beta)}{N^2}  \mathbb{E}\|\sum_{i=1}^N \mathcal{C}_\delta (\nabla f_i(x_{t-1}^i,\xi_{t-1}^i))\|^2. \nonumber
\end{eqnarray}
Further, we have that
\begin{eqnarray}\label{lemma4_2}
\mathbb{E}\|e_t\|^2 &=& (1-\delta)(1+\beta) \mathbb{E}\|e_{t-1}\|^2 + \frac{(1-\delta)(1+1/\beta)}{N^2}\bigg(\sum_{i=1}^N \mathbb{E}\|\mathcal{C}_\delta (\nabla f_i(x_{t-1}^i,\xi_{t-1}^i))\|^2 \nonumber \\
&&+ \sum_{i \neq j} \mathbb{E} \langle \mathcal{C}_\delta (\nabla f_i(x_{t-1}^i,\xi_{t-1}^i)), \mathcal{C}_\delta (\nabla f_i(x_{t-1}^j,\xi_{t-1}^j)) \rangle \bigg)\nonumber \\
&\leq& (1-\delta)(1+\beta) \mathbb{E}\|e_{t-1}\|^2 + \frac{(1-\delta)(1+1/\beta)}{N^2}\bigg(\sum_{i=1}^N \mathbb{E}\|\mathcal{C}_\delta(\nabla f_i(x_{t-1}^i,\xi_{t-1}^i)) \nonumber \\
&&-\nabla f_i(x_{t-1}^i,\xi_{t-1}^i)+\nabla f_i(x_{t-1}^i,\xi_{t-1}^i)\|^2+ \delta^2\sum_{i \neq j} \mathbb{E} \langle \nabla f_i(x_{t-1}^i,\xi_{t-1}^i), \nabla f_i(x_{t-1}^j,\xi_{t-1}^j) \rangle \bigg)\nonumber \\
&\leq& (1-\delta)(1+\beta) \mathbb{E}\|e_{t-1}\|^2 + \frac{(1-\delta)(1+1/\beta)}{N^2}\bigg(2(2-\delta)N M^2 \nonumber \\
&&+ \delta^2\sum_{i \neq j} \mathbb{E} \|\nabla f_i(x_{t-1}^i,\xi_{t-1}^i)\| \|\nabla f_i(x_{t-1}^j,\xi_{t-1}^j)\| \bigg)\nonumber \\
&=& (1-\delta)(1+\beta) \mathbb{E}\|e_{t-1}\|^2 + \frac{(1-\delta)(1+1/\beta)}{N^2}\bigg(2(2-\delta)N M^2 \nonumber \\
&&+ \delta^2\sum_{i \neq j} \mathbb{E} \|\nabla f_i(x_{t-1}^i,\xi_{t-1}^i)\|\mathbb{E} \|\nabla f_i(x_{t-1}^j,\xi_{t-1}^j)\| \bigg)\nonumber \\
&\leq& (1-\delta)(1+\beta) \mathbb{E}\|e_{t-1}\|^2 + \frac{(1-\delta)(1+1/\beta)}{N^2}\bigg(2(2-\delta)N M^2+ \delta^2 N (N-1) M^2 \bigg)\nonumber \\
&\leq& \frac{(1-\delta)(1+1/\beta)(2(2-\delta)+\delta^2 (N-1))M^2}{(1-(1-\delta)(1+\beta))N} \nonumber \\
&\leq& \frac{4(1-\delta)(2(2-\delta)+\delta^2 (N-1))M^2}{\delta^2 N}. \nonumber
\end{eqnarray}
where the first inequality comes from Assumption~\ref{assu4}. The second and third inequality follows from Assumption~\ref{assu3}. The last inequality holds by setting $\beta = \frac{\delta}{2(1-\delta)}$.
\end{proof}

\textbf{Proof of Lemma~\ref{lemma5}}
\begin{proof}
Similar to the proof of Lemma~\ref{lemma2}, we have that
\begin{eqnarray}\label{lemma5_1}
&&\sum_{i=1}^N \mathbb{E}\|\Bar{x}_t-x_t^i\|^2 \nonumber \\
&\leq& \eta^2 \sum_{i=1}^N \mathbb{E}\|\sum_{\tau=t'}^{t-1}\nabla f_i(x_\tau^i,\xi_\tau^i)-\mathcal{C}_\delta(\nabla f_i(x_\tau^i,\xi_\tau^i))\|^2.\nonumber \nonumber \\
&=& \eta^2 \sum_{i=1}^N \bigg( \sum_{\tau=t'}^{t-1} \mathbb{E}\|\nabla f_i(x_\tau^i,\xi_\tau^i)-\mathcal{C}_\delta(\nabla f_i(x_\tau^i,\xi_\tau^i))\|^2 \nonumber \\
&&+ \sum_{p \neq q} \langle \nabla f_i(x_p^i,\xi_p^i)-\mathcal{C}_\delta(\nabla f_i(x_p^i,\xi_p^i)), \nabla f_i(x_q^i,\xi_q^i)-\mathcal{C}_\delta(\nabla f_i(x_q^i,\xi_q^i)) \rangle \bigg) \nonumber \\
&\leq& \eta^2 \sum_{i=1}^N \bigg( (1-\delta)\sum_{\tau=t'}^{t-1} \mathbb{E}\|\nabla f_i(x_\tau^i,\xi_\tau^i)\|^2 + (1-\delta)^2 \sum_{p \neq q} \langle \nabla f_i(x_p^i,\xi_p^i), \nabla f_i(x_q^i,\xi_q^i) \rangle \bigg) \nonumber \\ 
&\leq& \eta^2 \sum_{i=1}^N \bigg( (1-\delta)(t-t') M^2 + (1-\delta)^2(t-t')(t-t'-1)M^2 \bigg) \nonumber
\end{eqnarray}
where the second inequality comes from the Definition~\ref{def1} and Assumption~\ref{assu4}. The third inequality follows from Assumption~\ref{assu3}. 
Thus, we have
\begin{eqnarray}
\frac{1}{N}\sum_{i=1}^N \mathbb{E}\|\Bar{x}_t-x_t^i\|^2 &\leq& \eta^2 \bigg( (1-\delta)(t-t') M^2 + (1-\delta)^2(t-t')(t-t'-1)M^2 \bigg) \nonumber \\
&\leq& \frac{(1-\delta)(1-\delta+\delta^2)}{\delta^2}\eta^2 M^2.
\end{eqnarray}
The last inequality holds because $t-t' \leq \lfloor \frac{1}{\delta} \rfloor \leq \frac{1}{\delta}$. 
\end{proof}

\textbf{Proof of Theorem~\ref{theo_2}}
\begin{proof}
Same to (\ref{theo1_3}) in the proof of Theorem~\ref{theo_1}, we have that
\begin{eqnarray}\label{theo2_1}
    \frac{\eta}{2}\sum_{t=0}^{T-1}\mathbb{E} \|\nabla f(\Bar{x}_t)\|^2 &\leq& f(x_0)-f(x^*) + \frac{\eta^3 L^2}{2} \sum_{t=0}^{T-1} \mathbb{E} \|e_t\|^2 + \frac{\eta L^2}{2N}  \sum_{t=0}^{T-1}  \sum_{i=1}^N \mathbb{E}\|\Bar{x}_t-x_t^i\|^2 \nonumber \\
    &&+ \frac{\eta^2 L}{2}\sum_{t=0}^{T-1} \mathbb{E} \|\frac{1}{N} \sum_{i=1}^{N} \nabla f_i(x_t^i,\xi_t^i)\|^2.
\end{eqnarray}
Substituting Lemma~\ref{lemma3}-\ref{lemma5} into (\ref{theo2_1}) yields that
\begin{eqnarray}
\frac{\eta}{2}\sum_{t=0}^{T-1} \mathbb{E}\|\nabla f(\Bar{x}_t)\|^2 &\leq& f(x_0)-f(x^*)+\frac{2(1-\delta)(2(2-\delta)+\delta^2 (N-1))\eta^3 L^2 M^2 T}{\delta^2 N} \nonumber \\
&&+ (\frac{\eta L^2}{2}+\eta^2 L^3)\frac{(1-\delta)(1-\delta+\delta^2)\eta^2 L^2 M^2}{\delta^2}\eta^2 M^2 T + \frac{\eta^2 L T \sigma^2}{2N} \nonumber \\
&&+ \eta^2 L \sum_{t=0}^{T-1} \|\nabla f(\Bar{x}_t)\|^2. \nonumber
\end{eqnarray}
Dividing by $\frac{\eta T}{2}$ on both sides of the above inequality and consider that $\eta L < \frac{1}{2}$, we obtain that
\begin{eqnarray}
    \frac{1-2\eta L}{T}\sum_{t=0}^{T-1} \mathbb{E} \|\nabla f(\Bar{x}_t)\|^2 &\leq&  \bigg(1-\delta+\delta^2+\frac{2(4+\delta^2(N-1))}{N}\bigg)\frac{2(1-\delta)\eta^2 L^2 M^2}{\delta^2}\nonumber \\
    &&+\frac{\eta L \sigma^2}{N} + \frac{2(f(x_0)-f^*)}{\eta T}. \nonumber
\end{eqnarray}

\end{proof}

\section{The Limitation of This Work}
Due to the limitation of computational resources, we do not verify the effectiveness of our proposed algorithm by training ultra-large deep learning models in the experiments. In addition, we also do not conduct the experiments in the environment with more than one node.

\section{Potential Negative Societal Impacts}
Our proposed algorithm is not immune to the risk of privacy leakage. Specifically, our algorithm needs to transmit the local model parameters and local stochastic gradients periodically. Thus, the attackers may infer the local data including the personal information and characteristics of the users in some practical applications. We would consider to solve the issue in future.
